# Supplementary material for: Imagery as Inquiry: Exploring A Multimodal Dataset for Conversational Recommendation
Source: arXiv:2405.14142 source file (2025-04-16)
Supplement: Supplementary file 1 [file appendix.tex]

\section{Appendix}
\label{sec:Appendix}

\subsection{Extracting Items from Comments}
\label{sec:Appendix:comments}

We use ChatGPT (gpt-3.5-turbo-0125) to extract items from comments. We use the following prompts for books and music, respectively:

\begin{quote}
In the following text, extract all books. Each book should be in the Author - Title format and separated by a newline. If an author is mentioned without the title, output the author only. If there are no mentions, output None.
\end{quote}

\begin{quote}
In the following text, extract all music tracks. Each track should be in the Artist - Title format and separated by a newline. If an artist is mentioned without the title, output the artist only. If there are no mentions, output None.
\end{quote}

We then further process the responses to get a list of items. The following are examples of comments to extracted items.

\begin{itemize}
    \item \textbf{Comment:} Book of A Thousand Days by Shannon Hale fits! It's one of my all-time favorites.\\
    $\rightarrow$ \textbf{Items:}  Shannon Hale - Book of A Thousand Days

    \item \textbf{Comment:} For some reason, the song You Get What You Give by New Radicals popped in my head when looking at this picture.\\
    $\rightarrow$ \textbf{Items:}  New Radicals - You Get What You Give

    \item \textbf{Comment:} Anything by Astro Man.\\
    $\rightarrow$ \textbf{Items:} Astro Man

    \item \textbf{Comment:} Lady of the Forest by Jennifer Roberson\\
    Rose Daughter and Spindle's End by Robin McKinley\\
    $\rightarrow$ \textbf{Items:}  Jennifer Roberson - Lady of the Forest, Robin McKinley - Rose Daughter, Robin McKinley - Spindle's End
\end{itemize}

\subsection{Statistics}
\label{sec:Appendix:statistics}
We obtain 1,470 requests and 12,208 items for \textit{books}; 796 requests and 38,204 items for \textit{music}. 
Each request has an average of $3.11$ ($\pm3.14$) images and $14.04$ ($\pm12.55$) recommended items for \textit{books}; $1.41$ ($\pm1.74$) images and $65.92$ ($\pm101.00$) items for \textit{music}.
Figure~\ref{fig:requests_per_year} shows the number of requests per year. There is a notable upward trend in the number of requests in both domains, with the counts for the initial two months of 2024 surpassing those of any full previous year.
Figure~\ref{fig:images_per_request} shows the number of images per request. 
Users tend to include multiple images for \textit{books}, while most use just one image for \textit{music}. 
Figure~\ref{fig:requests_per_year} plots the number of recommended items per request, showing long-tail distributions.
It's not unusual to see requests receive recommendations for dozens of items, and specifically in \textit{music}, some requests can accumulate more than a hundred items.

\begin{figure}[t]
    \centering
    \vspace{1em}
    \includegraphics[width=0.7\linewidth]{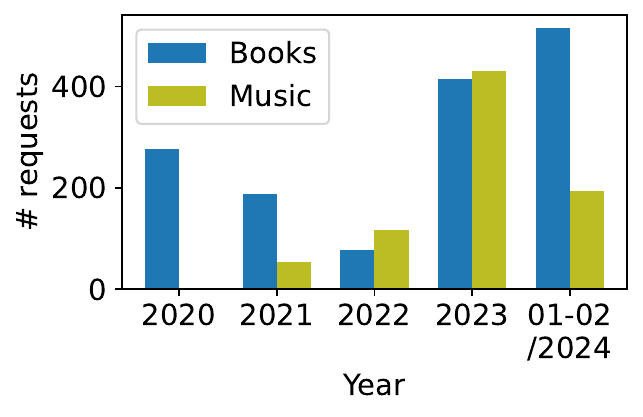}
    \caption{Requests per year}
    \label{fig:requests_per_year}
\end{figure}

\begin{figure}[ht]
    \centering
    \begin{subfigure}{0.5\linewidth}
        \centering
        \includegraphics[width=\linewidth]{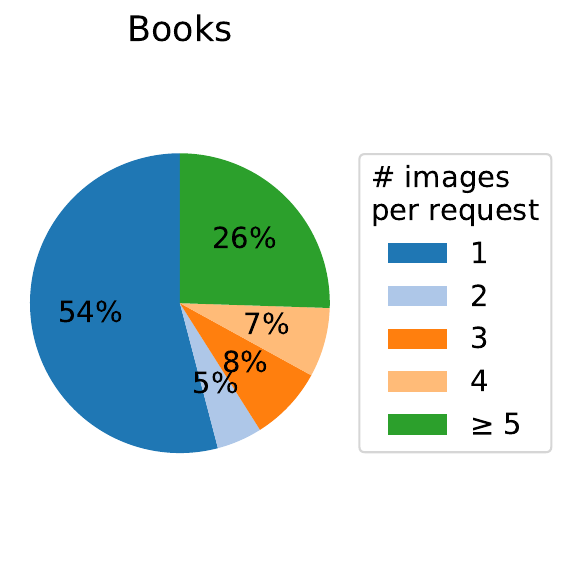}
        % \caption{\textit{Books}}
    \end{subfigure}%
    \begin{subfigure}{0.5\linewidth}
        \centering
        \includegraphics[width=\linewidth]{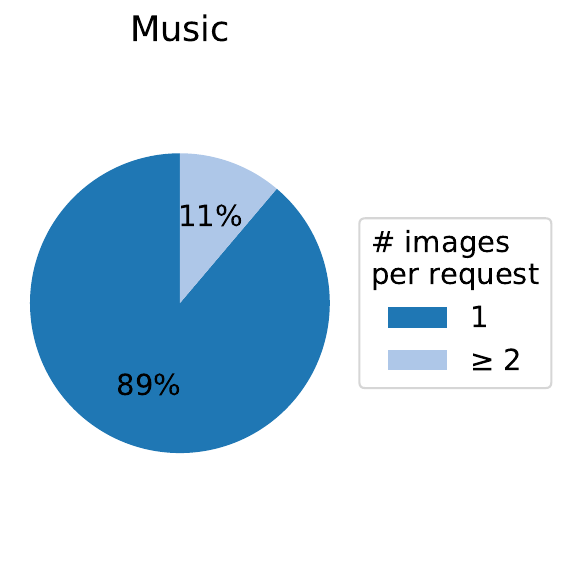}
        % \caption{\textit{Music}}
    \end{subfigure}
    \caption{Images per request}
    \label{fig:images_per_request}
\end{figure}

\begin{figure}[t]
    \centering
    \vspace{1em}
    \includegraphics[width=0.9\linewidth]{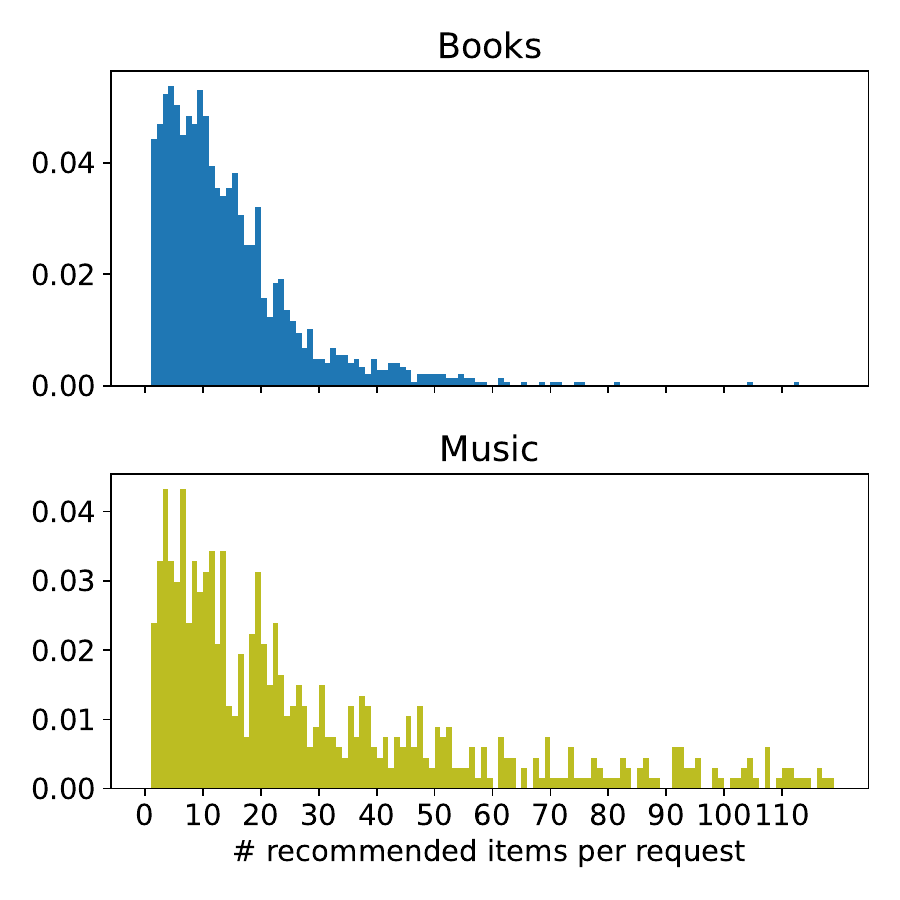}
    \caption{Recommended items per request}
    \label{fig:items_per_request}
\end{figure}

\subsection{Prompts}
\label{sec:Appendix:prompts}

We enlist all the prompts we use in our tasks.

\subsubsection{Title generation: standard prompting (books)}
\begin{quote}
Given the request, provide recommendations. Enumerate 20 books (1., 2., ...) in the order of relevance. Each book should take the Author - Title format. Don't say anything else.
\end{quote}

\subsubsection{Title generation: standard prompting (music)}
\begin{quote}
Given the request, provide recommendations. Enumerate 20 music pieces (1., 2., ...) in the order of relevance. Each piece should take the Artist - Title format. Don't say anything else.
\end{quote}

\subsubsection{Title generation: CoI prompting (books)}
\begin{quote}
Given the request, provide recommendations. Think step by step. First understand the given image(s) in detail, including its content, style, and vibe. Then, think of books that capture the essence of the image(s). Enumerate 20 books (1., 2., ...) in the order of relevance. Each book should take the Author - Title format. Don't say anything else.
\end{quote}

\subsubsection{Title generation: CoI prompting (music)}
\begin{quote}
Given the request, provide recommendations. Think step by step. First understand the given image(s) in detail, including its content, style, and vibe. Then, think of music pieces that capture the essence of the image(s). Enumerate 20 music pieces (1., 2., ...) in the order of relevance. Each piece should take the Artist - Title format. Don't say anything else.
\end{quote}

\subsubsection{Multiple-choice selection: standard prompting}

\begin{quote}
Given the request, choose which recommendation is the most suitable. Choose a single item. Don't say anything else.
\end{quote}

\subsubsection{Multiple-choice selection: CoI prompting}

\begin{quote}
Given the request, choose which recommendation is the most suitable. Think step by step. First understand the given image(s) in detail, including its content, style, and vibe. Then, carefully inspect each choice. Recall its content and see if it captures the essence of the image(s). Select the item that best captures this essence. Choose a single item. Don't say anything else.
\end{quote}

\subsection{More results}

We summarize all results for title generation in Figure~\ref{fig:all-generation}, multiple-choice selection in Figure~\ref{fig:all-selection}, and chain-of-imagery (CoI) prompting for text-only GPT-4 in Table~\ref{table:coi-additional}.
These results contain the information that support the takeaway messages of the paper:
\begin{enumerate}
    \item [M1] Models struggle, particularly smaller ones.
    \item [M2] Only larger models benefit from detailed descriptions.
    \item [M3] Using descriptions can be better than using images.
    \item [M4] Chain-of-imagery (CoI) prompting may help VLMs better harness their visual capabilities.
\end{enumerate}

Please refer to the main paper for detailed explanations of each.
 
\begin{figure}[t!]
    \centering
    \vspace{1em}
    \includegraphics[width=\linewidth]{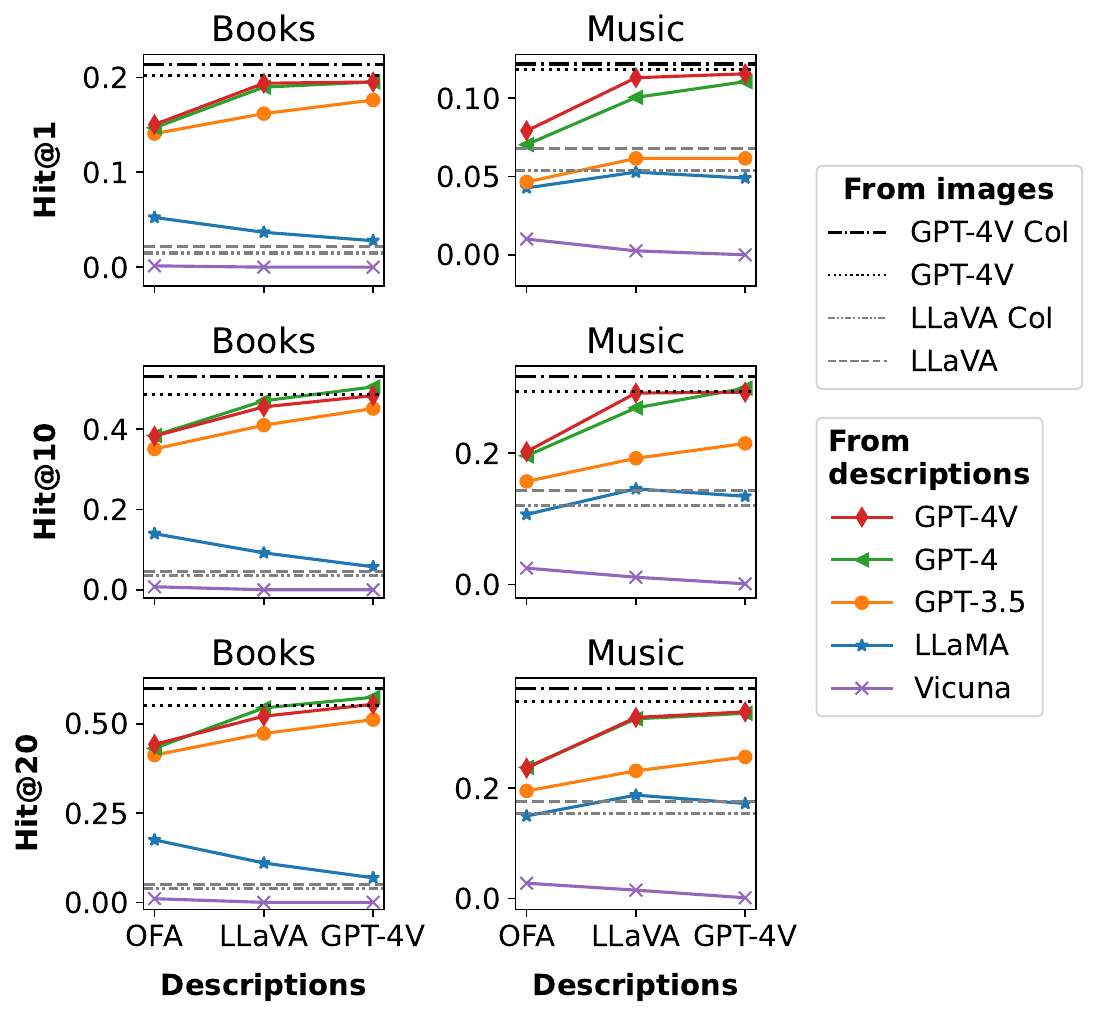}
    \caption{Results for title generation. Each row shows Hit@1, Hit@10, Hit@20 results, and each column shows \textit{books} and \textit{music} datasets, respectively. Vision models that take images as input are plotted in constant dotted lines; models that use only text descriptions (including GPT-4V without image input) are marked based on the type of description (x-axis).}
    \label{fig:all-generation}
\end{figure}

\begin{figure}[t!]
    \centering
    \vspace{1em}
    \includegraphics[width=\linewidth]{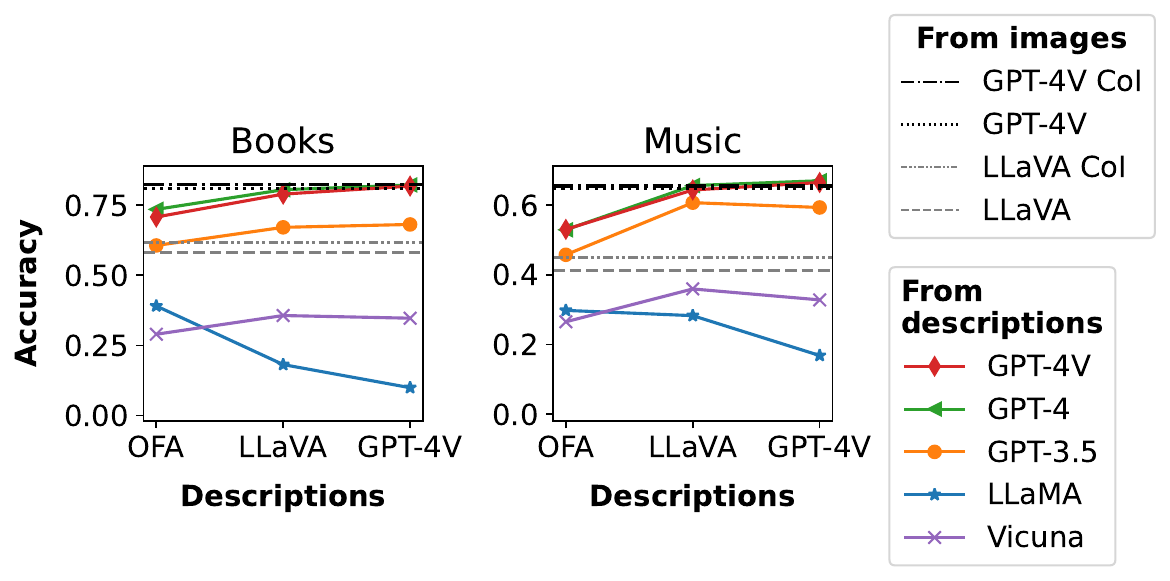}
    \caption{Results for multiple-choice selection. The plots are drawn in a similar style as in Figure~\ref{fig:all-generation}.}
    \label{fig:all-selection}
\end{figure}

\begin{table}[t!]
\centering
\caption{Chain-of-imagery (CoI) prompting results for \textit{text-only} GPT-4 (from GPT-4V descriptions). Unlike in the case of GPT-4V (from images), CoI does not always improve results.}
\label{table:coi-additional}
\begin{tabularx}{\columnwidth}{llcccc}
\toprule
\textbf{Dataset} & \textbf{Model} & \textbf{Hit@1} & \textbf{@10} & \textbf{@20} & \textbf{Acc (\%)} \\ 
\midrule
Books   
        & GPT-4 + CoI  & .2034 &  .5102 & .5946 & 81.70 \\
        & GPT-4        & .1952 & .5048 & .5741 & 82.18 \\
\midrule
Music   
        & GPT-4  & .0867 & .2663 & .3077 &  66.45 \\
        & GPT-4  & .1005 & .2990 & .3354 & 66.96 \\
\bottomrule
\end{tabularx}
\end{table}
